# Supplementary material for: Can't make an Omelette without Breaking some Eggs: Plausible Action Anticipation using Large Video-Language Models
Source: arXiv:2405.20305 source file (2024-05-30)
Supplement: Supplementary file 5 [file supp_dnr_ek100.tex]

\begin{table}[]
\centering
\begin{tabular}{l|ccc}
\hline
\multicolumn{1}{c|}{\multirow{2}{*}{\textbf{Method}}}          & \multicolumn{3}{c}{\textbf{\begin{tabular}[c]{@{}c@{}}Class-mean \\ Top-5 recall (\%) $\uparrow$\end{tabular}}} \\ \cline{2-4} 
\multicolumn{1}{c|}{} & \textbf{Verb}                           & \textbf{Noun}                          & \textbf{Action}                          \\ \hline
 % Video-LLaMA~\cite{zhang2023video} & 52.90 & 52.01 & 26.05 \\
\begin{tabular}[c]{@{}l@{}}PlausiVL (w/ DNR)\end{tabular} & 54.30 & 53.20 & 26.63                                      \\ 
PlausiVL   &   55.62  &  54.23   & 27.60 \\ \hline
\end{tabular}
\caption{(\epickitchens)~Performance of \method with and without "DNR: Do NOT repeat actions" in the prompt. Having DNR in the prompt is less effective than training the model with long-horizon action repetition loss~($\Lrep$) as objective function.}
\vspace{-2mm}
\label{tbl:dnr_ek100}
\end{table}
